# Supplementary material for: The three channels of many-body perturbation theory: $GW$, particle-particle, and electron-hole $T$-matrix self-energies
Source: arXiv:2309.04167 ancillary file (2024-02-29)
Supplement: Supplementary file 1 [file sup_ehT.pdf]

# Supplemntary Material for "The three channels of many-body perturbation theory: $GW$, particle-particle, and electron-hole $T$-matrix self-energies"

Roberto Orlando,[1,2,3] Pina Romaniello,[2,3,a)] and Pierre-François Loos[1,b)]
[1)] *Laboratoire de Chimie et Physique Quantiques, Université de Toulouse, CNRS, UPS, France*
[2)] *Laboratoire de Physique Théorique, Université de Toulouse, CNRS, UPS, France*
[3)] *European Theoretical Spectroscopy Facility (ETSF)*

Additional data regarding this manuscript can be found at https://github.com/pfloos/ehT.

## I. DERIVATION OF RPA-LIKE EQUATION FOR THE ELECTRON-HOLE $T$-MATRIX

Here, we derive the explicit expressions of the elements of the electron-hole (eh) $T$-matrix and the corresponding self-energy elements. A similar derivation can be carried out for the $GW$ and the particle-particle (pp) $T$-matrix approximations, and one ends up with the results already reported in the literature (see, for example, Refs. 1–4).

The eh $T$-matrix self-energy is defined as

$$\overline{\Sigma}^{\text{eh}}(12) = \text{i}G(43)T^{\text{eh}}(13;24) \tag{1}$$

with

$$T^{\text{eh}}(12;1'2') = -\overline{V}(12;1'2') - V(12';34)\overline{P}^{\text{eh}}(36;45)T^{\text{eh}}(52;1'6) \tag{2}$$

Our goal is to express the eh $T$-matrix in terms of a RPA-like response function. To do so, we first analyze its polarizability $\overline{P}^{\text{eh}}$ defined by

$$\overline{P}^{\text{eh}}(12;1'2') = -\text{i}G(12')G(21') \tag{3}$$

In the following, for the sake of simplicity, we drop the time dependence in the notation. Hence, one gets

$$\overline{P}^{\text{eh}}(\boldsymbol{x}_1,\boldsymbol{x}_4,\boldsymbol{x}_2,\boldsymbol{x}_3) = -\text{i}\sum_{pqrs}\varphi_p(\boldsymbol{x}_1)G_{pq}\varphi_q^*(\boldsymbol{x}_3)\varphi_r(\boldsymbol{x}_4)G_{rs}\varphi_s^*(\boldsymbol{x}_2) \tag{4}$$

from which

$$\overline{P}^{\text{eh}}_{pqrs} = \int d\boldsymbol{x}_1 d\boldsymbol{x}_2 d\boldsymbol{x}_3 d\boldsymbol{x}_4 \overline{P}^{\text{eh}}(\boldsymbol{x}_1,\boldsymbol{x}_4,\boldsymbol{x}_2,\boldsymbol{x}_3)\varphi_p^*(\boldsymbol{x}_1)\varphi_q(\boldsymbol{x}_3)\varphi_r^*(\boldsymbol{x}_4)\varphi_s(\boldsymbol{x}_2) = \overline{P}^{\text{eh}}_{(sp)(rq)} \tag{5}$$

We now use the following change of basis

$$T^{\text{eh}}_{npmo} = \int d\boldsymbol{x}_1 d\boldsymbol{x}_5 d\boldsymbol{x}_{1'} d\boldsymbol{x}_2 \varphi_n^*(\boldsymbol{x}_1)\varphi_p^*(\boldsymbol{x}_5)\varphi_m(\boldsymbol{x}_{1'})\varphi_o(\boldsymbol{x}_2)T^{\text{eh}}(\boldsymbol{x}_1,\boldsymbol{x}_5,\boldsymbol{x}_{1'}\boldsymbol{x}_2) \tag{6}$$

which yields

$$T^{\text{eh}}_{npmo} = -\overline{v}_{npmo} - \sum_{rstv} v_{nvro}\overline{P}^{\text{eh}}_{rstv}T^{\text{eh}}_{spmt} \tag{7}$$

or, in matrix form, we have

$$T^{\text{eh}}_{(on)(pm)} = -\overline{v}_{(on)(pm)} - \sum_{(vr)(ts)} v_{(on)(vr)}\overline{P}^{\text{eh}}_{(vr)(ts)}T^{\text{eh}}_{(ts)(pm)} \tag{8}$$

with the elements $v_{(on)(vr)} = v_{nvro}$ defined as

$$v_{pqrs} = \iint \frac{\varphi_p(\boldsymbol{x}_1)\varphi_q(\boldsymbol{x}_2)\varphi_r(\boldsymbol{x}_1)\varphi_s(\boldsymbol{x}_2)}{|\boldsymbol{r}_1 - \boldsymbol{r}_2|} d\boldsymbol{x}_1 d\boldsymbol{x}_2 \tag{9}$$

---

[a)] Electronic mail: pina.romaniello@irsamc.ups-tlse.fr
[b)] Electronic mail: loos@irsamc.ups-tlse.fr

We can now write

$$\sum_{(ts)}\underbrace{\left[\delta_{(on)(ts)}+\sum_{(vr)}v_{(on)(vr)}\overline{P}^{\text{eh}}_{(vr)(ts)}\right]}_{M_{(on)(ts)}}T^{\text{eh}}_{(ts)(pm)}=-\bar{v}_{(on)(pm)} \tag{10}$$

from which

$$T^{\text{eh}}_{(ts)(pm)}=-\sum_{(on)}M^{-1}_{(ts)(on)}\bar{v}_{(on)(pm)} \tag{11}$$

Using Eq. (11) in the right-hand side of Eq. (8), we arrive at

$$\begin{aligned}T^{\text{eh}}_{(on)(pm)}&=-\bar{v}_{(on)(pm)}+\sum_{(vr)(ts)(o'n')}v_{(on)(vr)}\overline{P}^{\text{eh}}_{(vr)(ts)}M^{-1}_{(ts)(o'n')}\bar{v}_{(o'n')(pm)}\\&=-\bar{v}_{(on)(pm)}+\sum_{(vr)(o'n')}v_{(on)(vr)}\overline{\chi}^{\text{eh}}_{(vr)(o'n')}\bar{v}_{(o'n')(pm)}\end{aligned} \tag{12}$$

where we have defined

$$\overline{\chi}^{\text{eh}}_{(vr)(o'n')}=\sum_{(ts)}\overline{P}^{\text{eh}}_{(vr)(ts)}M^{-1}_{(ts)(o'n')} \tag{13}$$

From this definition, one gets

$$\begin{aligned}\overline{P}^{\text{eh}}_{(vr)(ts)}&=\sum_{(o'n')}\overline{\chi}^{\text{eh}}_{(vr)(o'n')}M_{(o'n')(ts)}\\&=\sum_{(o'n')}\overline{\chi}^{\text{eh}}_{(vr)(o'n')}\left[\delta_{(o'n')(ts)}+\sum_{(v'r')}v_{(o'n')(v'r')}\overline{P}^{\text{eh}}_{(v'r')(ts)}\right]\\&=\overline{\chi}^{\text{eh}}_{(vr)(ts)}+\sum_{(o'n')(v'r')}\overline{\chi}^{\text{eh}}_{(vr)(o'n')}v_{(o'n')(v'r')}\overline{P}^{\text{eh}}_{(v'r')(ts)},\end{aligned} \tag{14}$$

which leads to

$$\left(\overline{\chi}^{\text{eh}}\right)^{-1}_{(vr)(ts)}=\left(\overline{P}^{\text{eh}}\right)^{-1}_{(vr)(ts)}+v_{(vr)(ts)} \tag{15}$$

Let us now look at the structure of $P$. From Eq. (3) and from the time structure of $T^{\text{eh}}$,[5] we have

$$\overline{P}^{\text{eh}}_{(vr)(ts)}(\omega)=-\mathrm{i}\int\frac{d\omega'}{2\pi}G_{rs}(\omega')G_{tv}(\omega'-\omega)e^{\mathrm{i}\omega'\eta} \tag{16}$$

Relying on the quasiparticle approximation of the one-body Green's function that reads

$$G(\boldsymbol{x}_1,\boldsymbol{x}_2;\omega)=\sum_{p}\frac{\varphi_p(\boldsymbol{x}_1)\varphi^*_p(\boldsymbol{x}_2)}{\omega-\epsilon_p+\mathrm{i}\eta\,\mathrm{sgn}(\epsilon_p-\mu)} \tag{17}$$

(where $\mu$ is the chemical potential), the polarizability $P$ then becomes

$$\overline{P}^{\text{eh}}_{(m'n)(n'm)}(\omega)=\frac{\delta_{nm}\delta_{n'm'}(f_n-f_{n'})}{(\epsilon_n-\epsilon_{n'})-\omega+\mathrm{i}\eta\,\mathrm{sgn}(\epsilon_{n'}-\epsilon_n)} \tag{18}$$

where $f_p=1$ if $\epsilon_p\leq\mu$ and 0 otherwise. Using expression (18) in Eq. (15), one ends up with

$$\overline{\chi}^{\text{eh}}_{(n_1n_2)(n_3n_4)}=\left[\delta_{nm}\delta_{n'm'}(\epsilon_n-\epsilon_{m'}-\omega)+(f_n-f_{m'})v_{(m'n)(n'm)}\right]^{-1}_{(n_1n_2)(n_3n_4)}(f_{n_4}-f_{n_3}) \tag{19}$$

which can be reformulated as an eigenvalue equation of the form

$$\begin{pmatrix} \overline{\boldsymbol{A}}^{\text{eh}} & \overline{\boldsymbol{B}}^{\text{eh}} \\ -\overline{\boldsymbol{B}}^{\text{eh}} & -\overline{\boldsymbol{A}}^{\text{eh}} \end{pmatrix} \begin{pmatrix} \overline{\boldsymbol{X}}^{\text{eh}} & \overline{\boldsymbol{Y}}^{\text{eh}} \\ \overline{\boldsymbol{Y}}^{\text{eh}} & \overline{\boldsymbol{X}}^{\text{eh}} \end{pmatrix} = \begin{pmatrix} \overline{\boldsymbol{X}}^{\text{eh}} & \overline{\boldsymbol{Y}}^{\text{eh}} \\ \overline{\boldsymbol{Y}}^{\text{eh}} & \overline{\boldsymbol{X}}^{\text{eh}} \end{pmatrix} \begin{pmatrix} \overline{\boldsymbol{\Omega}}^{\text{eh}} & \boldsymbol{0} \\ \boldsymbol{0} & -\overline{\boldsymbol{\Omega}}^{\text{eh}} \end{pmatrix} \tag{20}$$

with matrix elements given by the following expressions:

$$\overline{A}^{\text{eh}}_{ia,jb} = (\epsilon_a - \epsilon_i)\delta_{ij}\delta_{ab} - v_{ibja} \tag{21a}$$

$$\overline{B}^{\text{eh}}_{ia,jb} = -v_{ijba} \tag{21b}$$

Let us now consider the response function $\overline{\chi}^{\text{eh}}$ in Eq. (12). This function is a four-point quantity in real space (unlike $\chi^{\text{eh}}$ that is used to build $W$), since it is related to $\overline{P}^{\text{eh}}(12;34) = -\mathrm{i}G(14)G(23)$. Its spectral representation is

$$\overline{\chi}^{\text{eh}}(\boldsymbol{x}_1,\boldsymbol{x}_2,\boldsymbol{x}_3,\boldsymbol{x}_4;\omega) = \lim_{\eta\to 0^+} \sum_m \left[ \frac{\rho_m(\boldsymbol{x}_1,\boldsymbol{x}_3)\rho_m^*(\boldsymbol{x}_4,\boldsymbol{x}_2)}{\omega - \overline{\Omega}^{\text{eh}}_m + \mathrm{i}\eta} - \frac{\rho_m(\boldsymbol{x}_2,\boldsymbol{x}_4)\rho_m^*(\boldsymbol{x}_3,\boldsymbol{x}_1)}{\omega + \overline{\Omega}^{\text{eh}}_m - \mathrm{i}\eta} \right] \tag{22}$$

with

$$\begin{aligned} \rho_m(\boldsymbol{x}_1,\boldsymbol{x}_2) &= \langle \Psi_0 | \hat{\psi}^\dagger(\boldsymbol{x}_2)\hat{\psi}(\boldsymbol{x}_1) | \Psi_m \rangle \\ &= \sum_{jb} \langle \Psi_0 | \hat{a}_j^\dagger \hat{a}_b | \Psi_m \rangle \, \varphi_b(\boldsymbol{x}_1)\varphi_j^*(\boldsymbol{x}_2) + \sum_{jb} \langle \Psi_0 | \hat{a}_b^\dagger \hat{a}_j | \Psi_m \rangle \, \varphi_j(\boldsymbol{x}_1)\varphi_b^*(\boldsymbol{x}_2) \\ &= \sum_{jb} \left[ \overline{X}^{\text{eh}}_{jb,m} \varphi_b(\boldsymbol{x}_1)\varphi_j^*(\boldsymbol{x}_2) + \overline{Y}^{\text{eh}}_{jb,m} \varphi_j(\boldsymbol{x}_1)\varphi_b^*(\boldsymbol{x}_2) \right] \end{aligned} \tag{23}$$

where

$$\overline{X}^{\text{eh}}_{jb,m} = \langle \Psi_0 | \hat{a}_j^\dagger \hat{a}_b | \Psi_m \rangle \qquad \overline{Y}^{\text{eh}}_{jb,m} = \langle \Psi_0 | \hat{a}_b^\dagger \hat{a}_j | \Psi_m \rangle \tag{24}$$

With this definition of $\rho_m$, we get

$$\begin{aligned} \chi_{(vr)(o'n')} &= \int d\boldsymbol{x}_1 d\boldsymbol{x}_2 d\boldsymbol{x}_3 d\boldsymbol{x}_4 \chi(\boldsymbol{x}_1,\boldsymbol{x}_2,\boldsymbol{x}_3,\boldsymbol{x}_4)\varphi_r^*(\boldsymbol{x}_1)\varphi_{n'}(\boldsymbol{x}_4)\varphi_{o'}^*(\boldsymbol{x}_2)\varphi_v(\boldsymbol{x}_3) \\ &= \int d\boldsymbol{x}_1 d\boldsymbol{x}_2 d\boldsymbol{x}_3 d\boldsymbol{x}_4 \lim_{\eta\to 0^+} \sum_m \Bigg[ \frac{\rho_m(\boldsymbol{x}_1,\boldsymbol{x}_3)\rho_m^*(\boldsymbol{x}_4,\boldsymbol{x}_2)\varphi_r^*(\boldsymbol{x}_1)\varphi_{n'}(\boldsymbol{x}_4)\varphi_{o'}^*(\boldsymbol{x}_2)\varphi_v(\boldsymbol{x}_3)}{\omega - \overline{\Omega}^{\text{eh}}_m + \mathrm{i}\eta} \\ &\quad - \frac{\rho_m(\boldsymbol{x}_2,\boldsymbol{x}_4)\rho_m^*(\boldsymbol{x}_3,\boldsymbol{x}_1)\varphi_r^*(\boldsymbol{x}_1)\varphi_{n'}(\boldsymbol{x}_4)\varphi_{o'}^*(\boldsymbol{x}_2)\varphi_v(\boldsymbol{x}_3)}{\omega + \overline{\Omega}^{\text{eh}}_m - \mathrm{i}\eta} \Bigg] \end{aligned} \tag{25}$$

We now substitute Eq. (25) in Eq. (12) to get

$$\begin{aligned} T^{\text{eh}}_{(on)(ps)} &= T^{\text{eh}}_{npso} \\ &= -\bar{v}_{npso} + \sum_{vro'n'} v_{nvro} \int d\boldsymbol{x}_1 d\boldsymbol{x}_2 d\boldsymbol{x}_3 d\boldsymbol{x}_4 \lim_{\eta\to 0^+} \sum_m \Bigg[ \frac{\rho_m(\boldsymbol{x}_1,\boldsymbol{x}_3)\rho_m^*(\boldsymbol{x}_4,\boldsymbol{x}_2)\varphi_r^*(\boldsymbol{x}_1)\varphi_{n'}(\boldsymbol{x}_4)\varphi_{o'}^*(\boldsymbol{x}_2)\varphi_v(\boldsymbol{x}_3)}{\omega - \overline{\Omega}^{\text{eh}}_m + \mathrm{i}\eta} \\ &\quad - \frac{\rho_m(\boldsymbol{x}_2,\boldsymbol{x}_4)\rho_m^*(\boldsymbol{x}_3,\boldsymbol{x}_1)\varphi_r^*(\boldsymbol{x}_1)\varphi_{n'}(\boldsymbol{x}_4)\varphi_{o'}^*(\boldsymbol{x}_2)\varphi_v(\boldsymbol{x}_3)}{\omega + \overline{\Omega}^{\text{eh}}_m - \mathrm{i}\eta} \Bigg] \bar{v}_{n'pso'} \end{aligned} \tag{26}$$

We now define

$$L^{\text{eh}}_{pq,m} = \iint d\boldsymbol{x}_1 d\boldsymbol{x}_2 \varphi_p^*(\boldsymbol{x}_1) \frac{\rho_m(\boldsymbol{x}_1,\boldsymbol{x}_2)}{|\boldsymbol{r}_1 - \boldsymbol{r}_2|} \varphi_q(\boldsymbol{x}_2) = \sum_{jb} \left( v_{pjbq} \overline{X}^{\text{eh}}_{jb,m} + v_{pbjq} \overline{Y}^{\text{eh}}_{jb,m} \right) \tag{27}$$

and

$$
\begin{aligned}
R^{\text{eh}}_{pq,m} &= \iint d\boldsymbol{x}_1 d\boldsymbol{x}_2 \varphi^*_p(\boldsymbol{x}_1) \frac{\rho_m(\boldsymbol{x}_1,\boldsymbol{x}_2)}{|\boldsymbol{r}_1-\boldsymbol{r}_2|}\varphi_q(\boldsymbol{x}_2) - \iint d\boldsymbol{x}_1 d\boldsymbol{x}_2 \varphi^*_p(\boldsymbol{x}_2) \frac{\rho_m(\boldsymbol{x}_1,\boldsymbol{x}_1)}{|\boldsymbol{r}_1-\boldsymbol{r}_2|}\varphi_q(\boldsymbol{x}_2) \\
&= \sum_{jb} \iint d\boldsymbol{x}_1 d\boldsymbol{x}_2 \frac{\varphi^*_p(\boldsymbol{x}_1)\varphi_q(\boldsymbol{x}_2)}{|\boldsymbol{r}_1-\boldsymbol{r}_2|}\left[\overline{X}^{\text{eh}}_{jb,m}\varphi_b(\boldsymbol{x}_1)\varphi^*_j(\boldsymbol{x}_2) + \overline{Y}^{\text{eh}}_{jb,m}\varphi_j(\boldsymbol{x}_1)\varphi^*_b(\boldsymbol{x}_2)\right] \\
&- \sum_{jb} \iint d\boldsymbol{x}_1 d\boldsymbol{x}_2 \frac{\varphi^*_p(\boldsymbol{x}_2)\varphi_q(\boldsymbol{x}_2)}{|\boldsymbol{r}_1-\boldsymbol{r}_2|}\left[\overline{X}^{\text{eh}}_{jb,m}\varphi_b(\boldsymbol{x}_1)\varphi^*_j(\boldsymbol{x}_1) + \overline{Y}^{\text{eh}}_{jb,m}\varphi_j(\boldsymbol{x}_1)\varphi^*_b(\boldsymbol{x}_1)\right] \\
&= \sum_{jb}\left(v_{pjbq}\overline{X}^{\text{eh}}_{jb,m} + v_{pbjq}\overline{Y}^{\text{eh}}_{jb,m}\right) - \sum_{jb} v_{pjqb}\left(\overline{X}^{\text{eh}}_{jb,m} + \overline{Y}^{\text{eh}}_{jb,m}\right) \\
&= \sum_{jb}\left(\overline{v}_{pjbq}\overline{X}^{\text{eh}}_{jb,m} + \overline{v}_{pbjq}\overline{Y}^{\text{eh}}_{jb,m}\right)
\end{aligned}
\tag{28}
$$

where the last two equalities in Eqs. (27) and (28) are true only for real orbitals, which is what we assume in this work.

Thanks to these definitions, Eq. (26) becomes

$$
T^{\text{eh}}_{pqrs}(\omega) = -\overline{v}_{pqrs} + \sum_m \left[\frac{L^{\text{eh}}_{ps,m}R^{\text{eh}}_{rq,m}}{\omega - \overline{\Omega}^{\text{eh}}_m + \mathrm{i}\eta} - \frac{L^{\text{eh}}_{sp}R^{\text{eh}}_{qr,m}}{\omega + \overline{\Omega}^{\text{eh}}_m - \mathrm{i}\eta}\right] \tag{29}
$$

and the correlation part of the self-energy

$$
\overline{\Sigma}^{\text{eh}}_{pq}(\omega) = \mathrm{i}\sum_{rs}\int \frac{d\omega'}{2\pi} G_{rs}(\omega')T^{\text{eh}}_{psqr}(\omega-\omega')e^{i\omega'\eta} \tag{30}
$$

becomes

$$
\overline{\Sigma}^{\text{eh}}_{\text{c},pq}(\omega) = \sum_{im}\frac{L^{\text{eh}}_{ip,m}R^{\text{eh}}_{iq,m}}{\omega - \epsilon_i + \overline{\Omega}^{\text{eh}}_m - \mathrm{i}\eta} + \sum_{am}\frac{L^{\text{eh}}_{pa,m}R^{\text{eh}}_{qa,m}}{\omega - \epsilon_a - \overline{\Omega}^{\text{eh}}_m + \mathrm{i}\eta} \tag{31}
$$

This concludes the derivation.


[1] M. J. van Setten, F. Weigend, and F. Evers, J. Chem. Theory Comput. **9**, 232 (2013).
[2] F. Bruneval, T. Rangel, S. M. Hamed, M. Shao, C. Yang, and J. B. Neaton, Comput. Phys. Commun. **208**, 149 (2016).
[3] D. Zhang, N. Q. Su, and W. Yang, J. Phys. Chem. Lett. **8**, 3223 (2017).
[4] C. J. C. Scott, O. J. Backhouse, and G. H. Booth, J. Chem. Phys. **158**, 124102 (2023).
[5] P. Romaniello, F. Bechstedt, and L. Reining, Phys. Rev. B **85**, 155131 (2012).
